# Supplementary material for: Materializing Knowledge Bases via Trigger Graphs
Source: arXiv:2102.02753 source file (2021-02-04)
Supplement: Supplementary file 1 [file kbdd.tex]

\thmkboundedness*
\begin{proof}
    Consider a program $P$ and some ${k \geq 0}$.
    We assume that the rules in $P$ are normalized (i.e, their bodies comprise exclusively either $\EP$- or $\IP$-predicates).
    Let ${G^{k} = \full{P}{k}}$ and let ${G^{k+1} = \full{P}{k+1}}$.
    Let ${G^{k} = (V^k,E^k)}$ and let ${G^{k+1} = (V^{k+1},E^{k+1})}$.
    Let ${\mathcal{T}^{k+1} = \component{G^{k+1}}{k+1}}$ and
    let $\mathcal{I}$ be the set comprising each instance in ${\instComp(\mathcal{T}^{k+1})}$.

    First, we prove the auxiliary lemmas \ref{lemma:kboundedness:isomorphic-instances} and \ref{lemma:kboundedness:latoms}.

    \begin{lemma}\label{lemma:kboundedness:isomorphic-instances}
		For each subset ${\{\tau^{k+1}_1, \dots, \tau^{k+1}_m\}}$ of $\mathcal{T}^{k+1}$
		and each base instance $B$, s.t.
             ${\bigcup \limits_{1 \leq j \leq m} g_j(\leaves(\tau^{k+1}_j)) = B}$,
		where for each ${1 \leq j \leq m}$, $g_j$ is a homomorphism from ${\leaves(\tau^{k+1}_j)}$
		into $B$,
	      there exists an instance ${B^{\ast} \in \instComp(\mathcal{T}^{k+1})}$ that is isomorphic to $B$.
    \end{lemma}
    \begin{proof}
		From line~\ref{alg:k-boundedness:instComp:subset:start} of Algorithm~\ref{alg:k-boundedness}, we can see that the procedure $\instComp$
		considers each subset ${\{\tau^{k+1}_1, \dots, \tau^{k+1}_m\}}$ of $\mathcal{T}^{k+1}$.
		Hence, in order to prove Lemma~\ref{lemma:kboundedness:isomorphic-instances}, it suffices to show that
		for each base instance $B$, s.t.
             ${\bigcup \limits_{1 \leq j \leq m} g_j(\leaves(\tau^{k+1}_j)) = B}$,
		where for each ${1 \leq j \leq m}$, $g_j$ is a homomorphism from ${\leaves(\tau^{k+1}_j)}$
		into $B$,
	      there exists an instance ${B^{\ast} \in \instComp(\mathcal{T}^{k+1})}$ that is isomorphic to $B$.
	      Since ${\domain{g_i} \cap \domain{g_j} = \emptyset}$, for each ${1 \leq i \leq m}$ and each ${1 \leq j \leq m}$, with
		${i \neq j}$, it follows that \eqref{eq:vars:Delta} holds
		\begin{align}
			\Delta &= \bigcup \limits_{1 \leq j \leq m} \leaves(\tau^{k+1}_j)											\label{eq:Delta}\\
			\variables{\Delta} &= \bigcup \limits_{1 \leq j \leq m} \variables{\leaves(\tau^{k+1}_j)}						\label{eq:vars:Delta}
		\end{align}
		Since Algorithm~\ref{alg:k-boundedness} considers the vector $\vec{x}$ of
		all variables in $\Delta$, line~\ref{alg:k-boundedness:instComp:x:init},
		since it considers all isomorphically different vectors in ${\vec{c} \in \Constants^{\vert \vec{x} \vert}}$,
		line~\ref{alg:k-boundedness:instComp:c:start} and since for each such vector
		it computes the homomorphism ${h = \bigcup \nolimits_{i=1}^{|\vec{x}|} \{x_i \mapsto c_i\}}$
		and adds $h(\Delta)$ to $\mathcal{I}$, line~\ref{alg:k-boundedness:instComp:h}, it follows that
		Lemma~\ref{lemma:kboundedness:isomorphic-instances} holds.
    \end{proof}

    \begin{lemma}\label{lemma:kboundedness:latoms}
        For each EG ${\tau \in \bigcup \limits_{d=1}^{k+1} \component{G^{k+1}}{d}}$ of depth ${d \leq k+1}$, each base instance $B$ and
	 each fact ${F \in \tau(B)}$ of derivation depth $d$, there exists a homomorphism $g$ from
	 ${\leaves(\tau)}$ into $B$, such that ${F = \tau(g(\leaves(\tau)))}$.
    \end{lemma}
    \begin{proof}
		Let $v$ be a node in $\tau$, such that ${v(B) = F}$.
		Let $r$ be the rule associated with $v$.
		To prove the claim, we show the following property, for each $d$, where ${0 \leq d \leq k+1}$:
		\begin{compactitem}
			\item $\phi$. for each fact $F$ of derivation depth $d$, there exists a homomorphism $g^d$
			from ${\leaves(\tau_{\preceq v})}$ into $B$, such that ${F \in \tau_{\preceq v}(g^d(\leaves(\tau_{\preceq v})))}$.
		\end{compactitem}
		For ${d=0}$, $\phi$ holds, since an EG $\tau$ of depth 0 is the empty graph and, hence ${\tau(B) = B}$.
		For ${d=1}$, since the rules in $P$ are normalized (i.e, their bodies comprise exclusively either $\EP$- or $\IP$-predicates),
		it follows that ${\tau_{\preceq v} = (\{v\},\{\})}$
		and that $r$ is an extensional rule.
		Since $r$ is an extensional rule,
		it follows that ${\leaves(\tau_{\preceq v})) = \rho(\body{r})}$, line~\ref{alg:k-boundedness:leaves:leaf:append}.
		Furthermore, due to Definition~\ref{definition:guided-chase},
		it follows that there exists a homomorphism from $\body{r}$ into $B$.
		Due to the above, $\phi$ holds for ${d=1}$.

		For ${d+1}$, where ${d > 1}$, and assuming that $\phi$ holds for $d$, the proof proceeds as follows.
		Since the rules in $P$ are normalized and since ${d > 1}$, it follows that
		the body of $r$ comprises only \IP-atoms.
		Since $G^{k+1}$ is a full EG, it follows that for each ${1 \leq j \leq n}$, there exists (only) one
		edge of the form ${u_j \rightarrow_j v}$ in $E^{k+1}$.
		Hence, from Definition~\ref{definition:guided-chase}, it follows that
		there exists some ${h = \bigcup \nolimits_{j = 1}^n \Hom_j}$, such that ${h_s(\head{r}) = F}$ and
		for each ${1 \leq j \leq n}$, ${\Hom_j : p_j(\vec{x}_j) \rightarrow u_j(\BI)}$.
		Let ${F_j = h_j(p_j(\vec{x}_j))}$, for each ${1 \leq j \leq n}$.
		Since for each ${1 \leq j \leq n}$, $\tau_{\preceq u_j}$ has depth ${\leq d}$
		and since $\phi$ holds for $d$,
		it follows that for each ${1 \leq j \leq n}$, there exists a homomorphism $g_j$
		from ${\leaves(\tau_{\preceq u_j})}$ into $B$, such that ${F \in \tau_{u_j}(g_j(\leaves(\tau_{\preceq u_j})))}$.
		Since ${u_j \rightarrow_j v \in E^{k+1}}$,
		since ${\edges{\tau_{\preceq v}} \supseteq \edges{\tau_{\preceq u_j}}}$, for each ${1 \leq j \leq n}$,
		and due to line~\ref{alg:k-boundedness:instComp:Phi:init} of Algorithm~\ref{alg:k-boundedness}, it follows that
		\begin{align}
			\leaves(\tau_{\preceq v}) = \bigcup \limits_{j=1}^n \leaves(\tau_{\preceq u_j})
		\end{align}
		Since the variables occurring in ${\leaves(\tau_{u_i})}$ are different from the ones occurring in
  		${\leaves(\tau_{\preceq u_j})}$, for each ${1 \leq i \leq n}$ and each ${1 \leq j \leq n}$, with ${i \neq j}$,
		and due to the above, it follows that ${g = \bigcup \limits_{j=1}^{n} g_j}$ is a homomorphism from
		$\leaves(\tau_{\preceq v})$ into $B$, such that ${F \in \tau_{\preceq v}(g(\leaves(\tau_{\preceq v})))}$.
		Hence, $\phi$ holds for ${d+1}$.
 		The above concludes the proof of Lemma~\ref{lemma:kboundedness:latoms}.
    \end{proof}

	Using Lemmas~\ref{lemma:kboundedness:isomorphic-instances} and \ref{lemma:kboundedness:latoms},
	we next show the following lemma.

    \begin{lemma}\label{lemma:kboundedness:graph-equivalence}
        ${G^k(B) \models G^{k+1}(B)}$ holds, for each instance $B$ iff
        ${G^k(B^{\ast}) \models G^{k+1}(B^{\ast})}$ holds, for each instance $B^{\ast} \in \mathcal{I}$.
    \end{lemma}
    \begin{proof}
        ($\Rightarrow$) This direction trivially holds.

        ($\Leftarrow$)
        Suppose that ${G^k(B^{\ast}) \models G^{k+1}(B^{\ast})}$ holds, for each instance $B^{\ast} \in \mathcal{I}$.
        Due to the above, it follows that for each $B^{\ast} \in \mathcal{I}$,
	  there exists a homomorphism $h$ from ${G^{k+1}(B^{\ast})}$ into ${G^k(B^{\ast})}$.

        The proof works by contradiction.
        Suppose that there exists an instance $B$, such that
        ${G^k(B) \not \models G^{k+1}(B)}$ holds.
        This means that there exist ${F_1,\dots,F_m}$ in ${G^{k+1}(B) \setminus G^k(B)}$,
	  such that there does not exist a homomorphism from
	  ${\bigcup \limits_{1 \leq j \leq m} F_j}$ into $G^k(B)$.
	  We refer to the above property as ($\ast$).

	  Let $\tau^{k+1}_j$ be an EG, such that
        ${F_j \in \tau^{k+1}_j(B)}$, for each ${1 \leq j \leq m}$.
	  Due to Lemma~\ref{lemma:kboundedness:latoms},
	  we know that for each $F_j$, for ${1 \leq j \leq m}$, there exists a homomorphism
	  $g_j$ from ${\rho_j = \leaves(\tau^{k+1}_j)}$ into $B$, such that ${F_j = \tau(g_j(\rho_j))}$.
	  Let ${B_j = g_j(\rho_j)}$, for each ${1 \leq j \leq m}$.
	  We refer to each $B_j$ as an \emph{instantiator} for $\tau^{k+1}_j$, for each ${1 \leq j \leq m}$.
	  Since ${B' = \bigcup \limits_{1 \leq j \leq m} B_j \subseteq B}$,
	  and due to the above, the following hold:
	  (i) ${\tau^{k+1}_j(B) = \tau^{k+1}_j(B')}$, for each ${1 \leq j \leq m}$
        and (ii) ${\tau^{k}(B') \subseteq \tau^{k}(B)}$,
        for each ${\tau^{k} \in G^{k+1}}$.
        Due to (i) and (ii), Property ($\ast$)
        can be restated as follows: there exist ${F_1,\dots,F_m}$ in ${G^{k+1}(B') \setminus G^k(B')}$,
	  such that there does not exist a homomorphism from
	  ${\bigcup \limits_{1 \leq j \leq m} F_j}$ into $G^k(B')$.
         We distinguish the cases:
	  \begin{compactitem}
		\item $\tau^{k+1}_{j_1} \neq  \tau^{k+1}_{j_2}$, ${\forall j_1, j_2}$ in ${\{1,\dots,m\}}$, s.t. ${j_1 \neq j_2}$.
	        Below we show that there exists an instance ${B^{\ast} \in \mathcal{I}}$
	        that is isomorphic to $B'$.
	        Note that by showing this, we reach a contradiction, since
	        according to the base assumptions we know that
	        for each ${B^{\ast} \in \mathcal{I}}$,
		  there exists a homomorphism $h$ from ${G^{k+1}(B^{\ast})}$ into ${G^k(B^{\ast})}$.
	        The proof proceeds as follows.
		  Since due to the above the following holds
		  \begin{align}
			B' = \bigcup \limits_{1 \leq j \leq m} B_j = \bigcup \limits_{1 \leq j \leq m} g_j(\rho_j)
		 \end{align}
		 and due to Lemma~\ref{lemma:kboundedness:isomorphic-instances}, we know that
		 there exists an instance ${B^{\ast} \in \instComp(\tau^{k+1}_1,\dots,\tau^{k+1}_n)}$ that is isomorphic to $B'$.

		\item ${\tau^{k+1}_{j_1} =  \tau^{k+1}_{j_2}}$, for some ${j_1, j_2}$ in ${\{1,\dots,m\}}$, s.t. ${j_1 \neq j_2}$.
		WLOG, let ${\mathcal{B}_1,\dots,\mathcal{B}_{n'}}$ be sets of instances, where ${n' \leq n}$,
		such that for each ${1 \leq l \leq n'}$, $\mathcal{B}_l$ comprises all instances from ${B_1, \dots, B_m}$
		that are instantiators for the same EG.
		Let ${\tau_i = (B_i^1,\dots,B_i^{n'})}$ be the $i$-th $n'$-ary tuple of instances from ${\mathcal{B}_1 \times \dots \times \mathcal{B}_{n'}}$,
		where ${1 \leq i \leq M}$.
		By employing a reasoning similar to the one applied to the previous case, we know that
		for each ${1 \leq i \leq M}$, ${C_i = \bigcup \limits_{l=1}^{n'} B_i^l}$ is isomorphic to some instance
		${B^{\ast}_i \in \mathcal{I}}$.
		Since for each ${1 \leq i \leq M}$, ${G^k(B^{\ast}_i) \models G^{k+1}(B^{\ast}_i)}$ holds due to the base assumptions,
		it follows that ${G^k(C_i) \models G^{k+1}(C_i)}$ holds, for each ${1 \leq i \leq M}$, and consequently,
		that ${G^k(\bigcup \limits_{i=1}^M C_i) \models G^{k+1}(\bigcup \limits_{i=1}^M C_i)}$ holds.
		Due to the above, we reach a contradiction, since ${\bigcup \limits_{i=1}^M C_i = B'}$ and since
		there does not exist a homomorphism from ${\bigcup \limits_{1 \leq j \leq m} F_j}$ into $G^k(B')$
		according to the base assumptions.
	  \end{compactitem}
	  The above concludes the proof of Lemma~\ref{lemma:kboundedness:graph-equivalence}.
    \end{proof}

    The proof of Theorem~\ref{theorem:kboundedness} follows easily from
    Definition~\ref{definition:rule-classes}, Theorem~\ref{lemma:kboundedness:chase-equivalence}
    and Lemma~\ref{lemma:kboundedness:graph-equivalence}.
\end{proof}
