# Supplementary material for: Materializing Knowledge Bases via Trigger Graphs
Source: arXiv:2102.02753 source file (2021-02-04)
Supplement: Supplementary file 2 [file nonempty.tex]

\thmnonempty*

\input{figures/rule-set-fes-fus-not-bdd}

\begin{proof} Let \P be the program containing all of the rules in
    Figure~\ref{figure:rule-set-fes-fus-not-bdd}.  We show that $\P \notin \Bdd$
    (Lemma~\ref{lemma:is-not-bdd}), $\P \in \Fes$ (Lemma~\ref{lemma:is-fes}),
    and $\P \in \Fus$ (Lemma~\ref{lemma:is-fus}).
Theorem~\ref{theorem:non-empty} is a corollary of these results.
\end{proof}

\begin{lemma}
\label{lemma:is-not-bdd}
The program \P from
    Figure~\ref{figure:rule-set-fes-fus-not-bdd} is not \Bdd.
\end{lemma}

\begin{proof}
Given some $k \geq 3$, let $\I_k = \{\FP{bh}(c_i, c_{i+1}) \mid 1 \leq i \leq k-1\}$ and $\KB_k = ( \P, \I_k )$.
We show that $\Step{i}{\K_k} \not \models \Step{i+1}{\K_k}$ for all $i \in \{0, \ldots,  2 + \lfloor \frac{k}{2} \rfloor\}$.
Therefore, $\P \notin \Bdd$.

\input{figures/chain}

By the definition of the standard chase, the first four sets of facts $\Step{0}{\K_k}$, $\Step{1}{\K_k}$, $\Step{2}{\K_k}$, and $\Step{3}{\K_k}$ in the equivalent chase sequence of the KB $\K_k$, and the chase of $\K_k$ are as follows.
\begin{align*}
\Step{0}{\K_k} = \{	&\FP{bh}(c_i, c_{i+1}) \mid 1 \leq i \leq k-1\} (= \I_k) \\
\Step{1}{\K_k} = \{	&\FP{PT}(c_i, n_i, c_{i+1}), \FP{RT}(c_i, n_i, c_{i+1}) \mid 1 \leq i \leq k-1\} \cup \Step{1}{\K_k} \\
\Step{2}{\K_k} = \{	&\FP{GH}(n_i, n_{i+1}) \mid 1 \leq i \leq k-2)\} \cup \Step{2}{\K_k} \\
\Step{3}{\K_k} = \{	&\FP{OT}(n_1, m_2, n_2)\} \cup \{\FP{OT}(n_i, m_{i+1}, n_{i+1}), \FP{OT}(n_i, c_{i+1}, n_{i+1}) \mid 2 \leq i \leq k-2\} \cup \Step{2}{\K_k} \\
\Chase{\K_k} = \{	&\{\FP{RT}(m_i, n_i, m_{i+1}) \mid 2 \leq i \leq k-2\} \cup \Step{3}{\K_k}
\end{align*}
For the sake of clarity, we bijectively rename the nulls occurring in the above sets.

The set \Step{3}{\K_k} and the chase of $\K_k$ are illustrated in Figure~\ref{figure:chain}.
%, illustrated in Figure~\ref{figure:chain}, is the set $\{\FP{RT}(m_i, n_i, m_{i+1}) \mid 2 \leq i \leq m_{k-2})\} \cup \Step{4}{\K_k}$.
Note that we have to apply the rules in \P to the chase step \Step{3}{\K_k} at least $\lfloor \frac{k}{2} \rfloor$ times to compute the chase of $\K_k$.
Therefore, $\Step{i}{\KB_k} \not \models \Chase{\KB_k}$ for all $i \in \{0, \ldots, 3 + \lfloor \frac{k}{2} \rfloor\}$.
\end{proof}

\begin{lemma}
\label{lemma:is-fes}
The program \P from
    Figure~\ref{figure:rule-set-fes-fus-not-bdd} is \Fes.
\end{lemma}
\begin{proof}
We verify that, for any given instance \I, the KB $\K = ( \P, \I )$ admits a finite universal model.
This implies that the core chase of $( P, \I )$ terminates \cite{chaserevisited} which, in turn, implies that the equivalent chase of $( P, \I )$ also terminates \cite{k-boundedness}.
Therefore, $P \in \Fes$.

Without loss of generality, we assume that the instance \I is connected.
%That is, we assume that the undirected graph $\{(c, d) \mid \FP{bh}(c, d) \in \I\}$ is connected.
Note that given some (possibly unconnected) instance $J$, we can compute a universal model for the KB $( \P, J )$ as follows:
\begin{enumerate}
\item Compute (exactly) one universal model for each KB $( P, J_C )$ with $J_C$ a component of $J$.
\item Compute the disjoint union of these models.
\end{enumerate}
The above computation of a universal model for $J$ is possible because (i) every rule in \P is connected and (ii) this program does not feature any constants.

\input{figures/cycle}

To verify that $\K = ( \P, \I )$ admits a finite universal model, we present a comprehensive case by case analysis.
In each of these cases we will compute this model via the application of some of the rules in \P in a given specified order.
By doing so, we know that the resulting structure is universal---i.e., we know that it can be homomorphically mapped into any model of $\K$.
We show that in each of the cases the resulting structure is indeed a model separately.
\begin{enumerate}
\item Let $\BI$ be a base instance of the form $\{\FP{bh}(c_i, c_{i+1}) \mid 1 \leq i \leq k\}$ with $k \geq 1$.
We define the following sets of facts.
\begin{align*}
\M_1 &= \eqref{rule:pt-rt}(\BI) \cup \BI \Big(= \{\FP{PT}(c_i, n_i, c_{i+1}), \FP{RT}(c_i, n_i, c_{i+1}) \mid 1 \leq i \leq k-1\} \cup \BI\Big) \\
\M_2 &= \eqref{rule:gh}(\M_1) \cup \M_1 \Big(= \{	\FP{GH}(n_i, n_{i+1}) \mid 1 \leq i \leq k-2)\} \cup \M_1\Big) \\
\M_3 &= \eqref{rule:ot-1}(\M_2) \cup \M_2 \Big(=  \{\FP{OT}(n_i, c_{i+1}, n_{i+1}) \mid 2 \leq i \leq k-2\} \cup \M_2\Big) \\
\M_4 &= \eqref{rule:ot-3}(\M_3) \cup \M_3 \Big(= \{\FP{OT}(n_1, m_2, n_2)\} \cup \M_3\Big) \\
\M^2_5 &= \eqref{rule:rt-ot}(\M_4) \cup \M_4 \Big(= \{\FP{RT}(m_2, n_2, m_3), \FP{OT}(n_2, m_3, n_3)\} \cup \M_4\Big) \\
\M^i_5 &= \eqref{rule:rt-ot}(\M_5^{i-1}) \cup \M_5^{i-1} \Big(= \{\FP{RT}(m_i, n_i, m_{i+1}), \FP{OT}(n_i, m_{i+1}, n_{i+1})\}\Big) \text{ for all } i \in \{3, \ldots, k-2 \}
\end{align*}
The set $\M^{k-2}_5$ is a model for \K.
This structure is illustrated in the lower part of Figure~\ref{figure:chain}.

\item Let $\BI$ be a base instance of the form $\{\FP{bh}(c_i, c_{i+1}) \mid 1 \leq i \leq k\}$ with $k \geq 1$ and $c_k = c_1$.
We define the following sets of facts.
\begin{align*}
\M_1 &= \eqref{rule:pt-rt}(\BI) \cup \BI \Big(= \{\FP{PT}(c_i, n_i, c_{i+1}), \FP{RT}(c_i, n_i, c_{i+1}) \mid 1 \leq i \leq k-1\} \cup \BI \Big) \\
\M_2 &= \eqref{rule:gh}(\M_1) \cup \M_1 \Big(=\{\FP{GH}(n_i, n_{i+1}) \mid 1 \leq i \leq k-2\} \cup \{\FP{GH}(n_{k-1}, n_1)\} \cup \M_1 \Big) \\
\M_3 &= \eqref{rule:ot-1}(\M_2) \cup \M_2 \Big(= \{\FP{OT}(n_i, c_{i+1}, n_{i+1}) \mid 1 \leq i \leq k-2\} \cup \{\FP{OT}(n_{k-1}, c_1, n_1)\} \Big)
\end{align*}
The set $\M_3$ is a model for \K.
This structure is illustrated in Figure~\ref{figure:cycle}.

%Note that the core of \Step{3}{\K} is a model of \K and hence, $\CF{\Step{3}{\K}}$ is the chase of \K.
%Both these sets, $\Step{3}{\K}$ and \Chase{\K} are illustrated in Figure~\ref{figure:cycle}.
%Note that $\Chase{\K} = \CF{\Step{3}{\K}}$ since $\Step{3}{\K} \models \Step{4}{\K}$.
%The set of facts \Step{3}{\K} is illustrated in Figure~\ref{figure:cycle}.
%\todo{Draw picture!}
\item Let $\BI$ be a base instance containing some constants $c$, $d$, and $e$ such that $c \neq d$, and either $\FP{hb}(c, e), \FP{hb}(d, e) \in \I$ or $\FP{hb}(e, c), \FP{hb}(e, d) \in \I$.
In this case, we can realise that the knowledge base $K = (P, \BI)$ is unsatisfiable due to the rules \eqref{rule:break-1} and \eqref{rule:break-2} by observing \Step{1}{K}.
\end{enumerate}
\end{proof}

\input{figures/graph-rule-dependencies}

\begin{lemma}
\label{lemma:is-fus}
The program \P from
    Figure~\ref{figure:rule-set-fes-fus-not-bdd} is \Fus.
\end{lemma}
\begin{proof}
To verify that the program \P is \Fus we show that, for any given query $\Query$, the Algorithm~1 from \cite{DBLP:journals/semweb/KonigLMT15} will always terminate.
The only rule in $P$ that may hinder termination is \eqref{rule:rt-ot}, as it is the only one that can introduce rewritings that may need to be rewritten against this rule again (note how this rule contains the predicate \FP{OT} in the body and the head).
All other rules produce rewritings that can only serve as inputs for different rules: see the graph of rule dependencies for \P in Figure~\ref{figure:rulesdep}.
Nevertheless, note that all atoms $\FP{OT}(t, u, v)$ in a rewriting $\Query'$ produced by applying \eqref{rule:rt-ot}  include the atom $\FP{GH}(t, v)$.
By rewriting $\Query'$ against \ref{rule:ot-3}, we get that $\Query'' = \Query' \setminus \FP{OT}(t, u, v)$ is also $\P$-rewriting for $\Query'$ such that $\Query'' \subseteq \Query'$ and hence, $\Query'$ itself can be removed from the cover.
\end{proof}
