# Supplementary material for: Materializing Knowledge Bases via Trigger Graphs
Source: arXiv:2102.02753 source file (2021-02-04)
Supplement: Supplementary file 3 [file TG-rewriting-example.tex]

\begin{example}
	We demonstrate the computation of EG-rewritings. 
	Consider the rules 
	\begin{align*}
		\rs(X_1,Y_1,Z_1) &\rightarrow \T(X_1,X_1,Y_1) \tag{$r_1$} \\
		\T(X_2,Y_2,Z_2) &\rightarrow \Rp(Y_2,Z_2) \tag{$r_2$}
	\end{align*}
	where $\rs$ is the only extensional predicate. 
	Assume an EG with nodes $u_1$ and $u_2$, where $u_i$ is associated with $r_i$.
	Finally, assume that there exists an edge from $u_1$ into $u_2$. 
	Consider the query ${Q=R(Y_2,Z_2)}$. To compute the EG-rewriting of $Q$ under ${G_{\preceq u_2}}$
	we first compute the MGU between $\head{r_2}$ and $Q$. Since this MGU is trivial 
	the result of the first inductive step is ${Q'=\T(X_2,Y_2,Z_2)}$. Due to the edge from $u_1$ into $u_2$,  
	we next compute the EG-rewriting of ${Q'}$ under ${G_{\preceq u_1}}$.
	The MGU $\theta$ between $\head{r_1}$ and ${Q'}$ is ${\{X_1 \mapsto Y_2, Y_1 \mapsto Z_2\}}$
	and ${\theta(\body{r_1})}$ is ${\rs(Y_2,Z_2,Z_1)}$.
	The EG-rewriting $Q^r$ of $u_2$ is given by ${\exists Z_1. \rs(Y_2,Z_2,Z_1)}$.
	We can see that for each answer $\sigma$ to $Q^r$ over $B$, 
	the fact ${\Rp(\sigma Y_2, \sigma Z_2)}$ is in ${u_2(B)}$.  
\end{example}
