# Supplementary material for: Materializing Knowledge Bases via Trigger Graphs
Source: arXiv:2102.02753 source file (2021-02-04)
Supplement: Supplementary file 4 [file table-benchmarks-depths.tex]

\begin{table}[tb]
    \centering
    \scriptsize
    \begin{adjustbox}{max width=\columnwidth}
            \begin{tabular}{ p{1cm} ccc}
                 \textbf{Scenario}        & LI & L & LE \\
                 \hline
                \multicolumn{4}{l}{\bf Linear and Datalog scenarios} \\
                LUBM & 6 & 4 & 5 \\
                UOBM & 9 & 6 & NA \\
                DBpedia & 17 & 8 & NA \\
                Claros & 23 & 9 & 9 \\
                React. & 8 & NA & NA \\
                \multicolumn{4}{l}{\bf ChaseBench scenarios} \\
                S-128 & NA & 2 & NA\\
                O-256 & NA & 3 & NA\\
                \multicolumn{4}{l}{\bf RDFS ($\rho$DF) scenarios} \\
                LUBM & NA & 4 & NA \\
                YAGO & NA & 20 & NA \\
            \end{tabular}
    \end{adjustbox}
    \caption{Maximum reasoning depth of the considered benchmarks.}
    \label{tab:benchmarks-depths}
\end{table}
