# Supplementary material for: Materializing Knowledge Bases via Trigger Graphs
Source: arXiv:2102.02753 source file (2021-02-04)
Supplement: Supplementary file 5 [file table-chasebench-multi.tex]

\begin{table*}[h]
    \centering
    \scriptsize
    \begin{adjustbox}{max width=\textwidth}
    {
    \begin{tabular}{ p{1.5cm}
            S[table-format=2.1,table-column-width=2.5cm]
            S[table-format=2.1,table-column-width=2.5cm]
            S[table-format=1.1,table-column-width=2.5cm]
        || S[table-format=1.1,table-column-width=1cm]
	  }
        & \multicolumn{3}{S[table-format=1.3,table-column-width=2.5cm]}{\textbf{RDFox}}
        & \multicolumn{1}{S[table-format=6.2,table-column-width=1.5cm]}{\textbf{GLog}~{no opt}}\\

        \textbf{Scenario}  & {Runtime (1 thread)} & {Runtime (8 threads)} & {Runtime (16 threads)} & {Runtime} \\

        \hline
        STB-128 & 13.4 & 2.9 & 2.3 	          & 0.2 \\
        ONT-256 & 49 & 10 & 7.8	          & 1 \\
    \end{tabular} }
    \end{adjustbox}
    \caption{\chaseBench scenarios. Time is in s.}
    \label{tab:chaseBench-multi}
\end{table*}
