# Supplementary material for: Materializing Knowledge Bases via Trigger Graphs
Source: arXiv:2102.02753 source file (2021-02-04)
Supplement: Supplementary file 6 [file table-chasebench-unopt.tex]

\begin{table*}[h]
    \centering
    \scriptsize
    \begin{adjustbox}{max width=\textwidth}
    {
    \begin{tabular}{ p{1.5cm}
            S[table-format=1.1,table-column-width=1cm]
            S[table-format=4,table-column-width=1cm]
        || S[table-format=2.1,table-column-width=1cm]
            S[table-format=4,table-column-width=1cm]
        || S[table-format=2,table-column-width=1cm]
            S[table-format=4,table-column-width=1cm]
        || S[table-format=2.1,table-column-width=1cm]
            S[table-format=2.1,table-column-width=1cm]
	  }
        & \multicolumn{2}{S[table-format=1.3,table-column-width=1.5cm]}{\textbf{VLog}}
        & \multicolumn{2}{S[table-format=1.3,table-column-width=1.5cm]}{\textbf{RDFox}}
        & \multicolumn{2}{S[table-format=1.3,table-column-width=1.5cm]}{\textbf{COM}}
        & \multicolumn{2}{S[table-format=6.2,table-column-width=1.5cm]}{\textbf{GLog}~{no opt}}\\

        \textbf{Scenario}  & {Runtime} & {Memory} & {Runtime} & {Memory} & {Runtime} & {Memory} & {Runtime} & {Memory} \\

        \hline
        STB-128 & 0.5  & 1350 			& 13.4 & X 		& 10      & X 	          & 0.2 & 1266 \\
        ONT-256 & 2.3 & 4930 			& 49 & X 		& 35    	& X 	          & 1 & 4929\\
    \end{tabular} }
    \end{adjustbox}
    \caption{\chaseBench scenarios. Time is in s and memory in MB.}
    \label{tab:chaseBench-unopt}
\end{table*}
