# Supplementary material for: Materializing Knowledge Bases via Trigger Graphs
Source: arXiv:2102.02753 source file (2021-02-04)
Supplement: Supplementary file 7 [file table-datalog-multi.tex]

\begin{table*}[h]
    \centering
    \scriptsize
    \begin{adjustbox}{max width=\textwidth}
    {
    \begin{tabular}{ p{1.5cm}
            S[table-format=4.1,table-column-width=2.5cm]
            S[table-format=3.1,table-column-width=2.5cm]
            S[table-format=3.1,table-column-width=2.5cm]
         || S[table-format=4.1,table-column-width=0.8cm]
           S[table-format=4.1,table-column-width=0.8cm]
           S[table-format=4.1,table-column-width=0.8cm]
        }
        & \multicolumn{3}{S[table-format=1.3,table-column-width=2.5cm]}{\textbf{RDFox}} 
        & \multicolumn{3}{S[table-format=6.2,table-column-width=1.5cm]}{\textbf{GLog Runtime}}\\

        \textbf{Scenario}  & {Runtime (1 thread)} & {Runtime (8 threads)} & {Runtime (16 threads)} & {No opt} & {m} & {m+r} \\

        \hline
        LUBM-L 	& 23 & 4.8 & 3.8 					&2.4 & 2.2 & 1.0                     \\
        LUBM-LE 	& 116.6 & 20.9 & 16.2 			& 17.3 & 17.2 & 16.1               \\
        UOBM-L 	& 10 & 2 & 1.6 					& 2.6 & 2.4 & 2.6                    \\
        DBpedia-L 	& 64.4 & 29 & 23.9 				& 20 & 19 & 19                       \\
        Claros-L 	& 2512 & 296 & 171.1 			& 122 & 118.3 & 119               \\
        Claros-LE   & * & * & * 						& 1040.8 & 1012.2 & 1053.9    \\
    \end{tabular} }
    \end{adjustbox}
    \caption{{Linear and Datalog scenarios. Time is in s. * denotes runtime exception.}}
    \label{tab:datalog-multi}
\end{table*}
