# Supplementary material for: Materializing Knowledge Bases via Trigger Graphs
Source: arXiv:2102.02753 source file (2021-02-04)
Supplement: Supplementary file 8 [file table-datalog-unopt.tex]

\begin{table*}[h]
    \centering
    \scriptsize
    \begin{adjustbox}{max width=\textwidth}
    {
    \begin{tabular}{ p{1.5cm}
            S[table-format=4.1,table-column-width=1cm]
            S[table-format=4,table-column-width=1cm]
        || S[table-format=4.1,table-column-width=1cm]
            S[table-format=4,table-column-width=1cm]
        || S[table-format=4.1,table-column-width=1cm]
            S[table-format=4,table-column-width=1cm]
        || S[table-format=4.1,table-column-width=0.8cm]
            S[table-format=4.1,table-column-width=0.8cm]
            S[table-format=4.1,table-column-width=0.8cm]
        || S[table-format=4,table-column-width=0.8cm]
           S[table-format=4,table-column-width=0.8cm]
           S[table-format=4,table-column-width=0.8cm]}
        & \multicolumn{2}{S[table-format=1.3,table-column-width=1.5cm]}{\textbf{VLog}}
        & \multicolumn{2}{S[table-format=1.3,table-column-width=1.5cm]}{\textbf{RDFox}}
        & \multicolumn{2}{S[table-format=1.3,table-column-width=1.5cm]}{\textbf{COM}}
        & \multicolumn{3}{S[table-format=6.2,table-column-width=1.5cm]}{\textbf{GLog Runtime}}
        & \multicolumn{3}{S[table-format=6.2,table-column-width=1.5cm]}{\textbf{GLog Memory}} \\

        \textbf{Scenario}  & {Runtime} & {Memory} & {Runtime} & {Memory} & {Runtime} & {Memory} & {No opt} & {m} & {m+r} & {No opt} & {m} & {m+r} \\

        \hline
        LUBM-L & 1.5 & 324 			& 23 & X 		& 20.4      & X 	          &  2.5 & 2.2 & 1             	 			&  446 & 424 & 265 \\
        LUBM-LE & 170.5 & 2725 		& 116.6 & X 		& 115.9    & X 	          &  71.1 &	68.8 &67.7              			&  2880	& 2688	& 2695 \\
        UOBM-L & 7.3& 1021 			& 10 & X 		& 10        & X 	          &  4.4 & 6.3 & 6.3               			&  506 & 590 & 590\\
        DBpedia-L & 41.6 & 827 			& 64.4 & X 		& 198.4    & X 	          & 31.4 &	32 &  31.1               			&  2335	& 2319 & 2313 \\
        Claros-L & 431 & 3170 			& 2512 & X 		& 2373.0  & X 	          &  128.6 & 125.6 &	126.7               		&  5954 & 5957	& 5958\\
        Claros-LE & 2771.8 & 11895 		& * & * 			& *          & * 	          &  1104.3	& 1094 & 1106.3  		   	&  48246 & 48251 & 48223 \\
    \end{tabular} }
    \end{adjustbox}
    \caption{{Linear and Datalog scenarios. Time is in s and memory in MB.}}
    \label{tab:datalog-unopt}
\end{table*}
