# Supplementary material for: Materializing Knowledge Bases via Trigger Graphs
Source: arXiv:2102.02753 source file (2021-02-04)
Supplement: Supplementary file 9 [file table-optimizations.tex]

\begin{table}[tb]
    \centering
    \scriptsize
    \begin{adjustbox}{max width=\columnwidth}
    {    
    \begin{tabular}{ p{1.6cm} S[table-format=1.4,table-column-width=0.8cm] S[table-format=2.2,table-column-width=0.8cm]}
        \textbf{Scenario} & m & r \\ 
        \hline
        LUBM-L & 0.0005 & 0.16 \\
        LUBM-LE & 0.0007 & 0.16 \\
        UOBM-L & 0.08 & 0.02 \\
        DBpedia-L & 0.05 & 0.5 \\
        Claros-L & 0.03 & 2.8 \\
        Claros-LE & 0.3 & 15.2\\
    \end{tabular} }
    \end{adjustbox}
    \caption{{Cost of optimizations.}}
    \label{tab:datalog-optimizations}
\end{table}
