# Supplementary material for: Materializing Knowledge Bases via Trigger Graphs
Source: arXiv:2102.02753 source file (2021-02-04)
Supplement: Supplementary file 10 [file table-rdfs-unopt.tex]

\begin{table*}[h]
    \centering
    \scriptsize
    \begin{adjustbox}{max width=\textwidth}
    {
    \begin{tabular}{ p{1.5cm}
            S[table-format=1.1,table-column-width=1cm]
            S[table-format=4,table-column-width=1cm]
        || S[table-format=2.1,table-column-width=1cm]
            S[table-format=4.1,table-column-width=1cm]
        || S[table-format=2.1,table-column-width=1cm]
            S[table-format=4.1,table-column-width=1cm]
        || S[table-format=4.1,table-column-width=0.8cm]
            S[table-format=4.1,table-column-width=0.8cm]
            S[table-format=4.1,table-column-width=0.8cm]
        || S[table-format=4,table-column-width=0.8cm]
           S[table-format=4,table-column-width=0.8cm]
           S[table-format=4,table-column-width=0.8cm]
	  }
        & \multicolumn{2}{S[table-format=1.3,table-column-width=1.5cm]}{\textbf{VLog}}
        & \multicolumn{2}{S[table-format=6.2,table-column-width=1.5cm]}{\textbf{WebPie}}
        & \multicolumn{2}{S[table-format=6.2,table-column-width=1.5cm]}{\textbf{Infearray}}
        & \multicolumn{3}{S[table-format=6.2,table-column-width=1.5cm]}{\textbf{GLog Runtime}}
        & \multicolumn{3}{S[table-format=6.2,table-column-width=1.5cm]}{\textbf{GLog Memory}}\\

        \textbf{Scenario}  & {Runtime} & {Memory} & {Runtime} & {Memory} & {Runtime} & {Memory} & {No opt} & {m} & {m+r} & {No opt} & {m} & {m+r} \\

        \hline
        LUBM & 0.1  & 189 				& 353  & 200  			& 23 & 2000 			& 0.4 &	0.4 & 0.3  		& 187 & 187	& 181 \\
        Yago & 163  & 3192 			& 808  & 200 			& 116.6 & 14000 		& X	& X & X 				& 1447 & 1600 &	1610 \\
    \end{tabular} }
    \end{adjustbox}
    \caption{{\chaseBench and RDFS scenarios. Time is in s and memory in MB.}}
    \label{tab:rdfs-unopt}
\end{table*}
